# Supplementary material for: Stay in Touch! Shape and Shadow Influence Surface Contact in XR Displays
Source: arXiv:2201.01889 source file (2022-01-06)
Supplement: Supplementary file 1 [file 7_Supplemental.tex]

%%%%%%%%%% Prefix a "S" to all equations, figures, tables and reset counters

\newcommand{\beginsupplement}{%
        \setcounter{page}{1}
        \setcounter{section}{0}
        \setcounter{figure}{0}
        \setcounter{table}{0}
        \setcounter{equation}{0}
        \renewcommand{\thetable}{S\arabic{table}}%
        \renewcommand{\thefigure}{S\arabic{figure}}%
        \renewcommand{\theequation}{S\arabic{equation}}
     }
     
\clearpage 
\pagebreak
\beginsupplement

% LAZY TITLE SOLUTION I KNOW. Maybe I'll make it nice later. But probably not. 
\begin{tabularx}{\textwidth}{X}
  \begin{center}
    \textbf{\huge Supplemental Materials: } \\
    \textbf{\huge Stay in Touch! Shape and Shadow Influence Surface Contact in XR Displays} \\  
    \vspace{3ex}
    \large\textup{Haley Adams, Holly Gagnon, Jeanine Stefanucci, Sarah Creem-Regehr, and Bobby Bodenheimer}
    \end{center} 
\end{tabularx}

%Haley Adams, Holly Gagnon, Jeanine Stefanucci, Sarah Creem-Regehr,and Bobby Bodenheimer,Member, IEEE

%Individual Data for Experiment 1
\section{Variance for Experiment 1}

% I calculated the ICC (amount of variance accounted for by the grouping variable (i.e., differences between participants)) and it's essentially 0, meaning that there isn't much variance between participants, so you don't need an RE

We evaluated to what extent between participant variance accounted for the variance in our collected data by calculating the intraclass correlation coefficient (ICC). The ICC measures the amount of variance accounted for by a grouping variable. For our analysis, individual participants was selected as the grouping variable, where an ICC value of 1 indicates  that  any  variance  in  the  data  is  between  participants  while  a  value  of  0  indicates  that  no  variance  in  the data is due to between participant factors. 

We found that $\tau_{ost}$ = 0.009 for data collected with the OST AR display, which indicates negligible variance was caused by between subjects factors. Similarly low ICC values were found for the VST AR  and VR display data with ICCs of $\tau_{vst}$ = 0.012 and $\tau_{vr}$ = 0.042, respectively. To supplement this calculation, we present the psychometric curves for each participant in Figure \ref{fig:sup:exp1_indivs}, as well.

\section{Individual Data for Experiment 2}

%All human things are subject to decay. And when fate summons, Monarchs must obey. 

%In the same manner
Using the same approach that we employed for Experiment 1, we evaluated the extent to which participant variance accounted for variance in our collected data by calculating the intraclass correlation coefficient (ICC) for Experiment 2. For the OST AR display condition we found $\tau_{ost}$ = 0.006 and for the VST AR display we found $\tau_{vst}$ = 0.028. For the VR display condition $\tau_{vr}$ = 0.023. Because our ICC values were near zero, we can understand that our experimental findings were not significantly influenced by between participant variation. We depict the psychometric curves for each participant in Figure \ref{fig:sup:exp2_indivs}.

% HoloLens: [1] 0.005867887
% Zed:      [1] 0.02776144
% VR:       [1] 0.02341385

%% NOTES FROM HOLLY
%% We need to use a binomial model, but it doesn't need to be mixed (i.e., doesn't need a random effect for participant). This is for a few reasons: %    1) You only have 6 "groups" (participants), and from my MLM class, it's recommended to have 20 groups to include an RE (including an RE for less than that isn't necessarily wrong, just not necessarily necessary); 
%    2) Your experiment was designed to minimize variance between individuals; and 
%    3) I calculated the ICC (amount of variance accounted for by the grouping variable (i.e., differences between participants)) and it's essentially 0, meaning that there isn't much variance between participants, so you don't need an RE

\section{Tables of Statistical Results}
\haley{These are temporary I guess! }
\holly{I keep looking at logistic regression papers, and there isn't much consistency as to which stats are reported in the table. We definitely want B and OR. I think to save space, it's easier to denote significance with an asterisk next to the B value and put a p-value key at the bottom of the table. Then I'm thinking we could include the SE and 95\% confidence interval. Currently, in the results section, I report the SE for the beta value (logit). If we want to report the CI, let me know if you think it would be more useful to have it be for the odds ratios. I can also go back and use the odds ratio SEs if that would be more informative. We also want to include all predictors in the table (e.g., instead of "Fixed Effect", the column name could be "Predictor"). The list of predictors would be: Intercept(Constant), Shadow, Cube, Icosahedron, Height, Shadow x Cube, Shadow x Icosahedron. In the table note, we would specify the reference groups.} \haley{Yes yes. These are good ideas. I'm going to whip up an example based on your ideas here. It also raises some questions though. Will talk about it during our meeting this afternoon!}

\input{tables/_Exp1_Tables}

\input{tables/_Exp2_Tables}
